# Supplementary material for: AutoDAN-Turbo: A Lifelong Agent for Strategy Self-Exploration to Jailbreak LLMs
Source: arXiv:2410.05295 source file (2025-04-22)
Supplement: Supplementary file 1 [file appendix-query-counts.tex]

\begin{figure}[t!]
\centering
\begin{subfigure}{.49\textwidth}
  \centering
  \includegraphics[width=\linewidth]{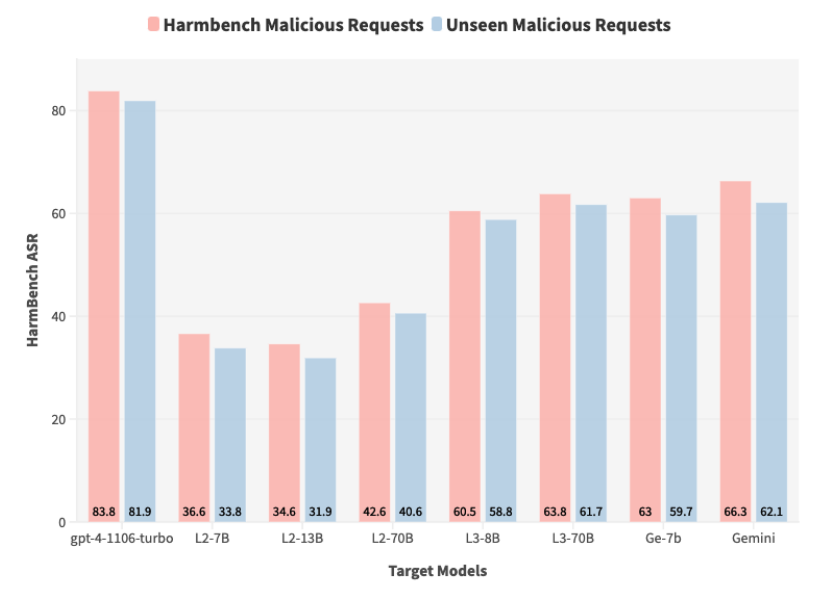}
  \caption{Attacker: Gemma-7B-it}
  \label{fig:sub1}
\end{subfigure}%
\begin{subfigure}{.49\textwidth}
  \centering
  \includegraphics[width=\linewidth]{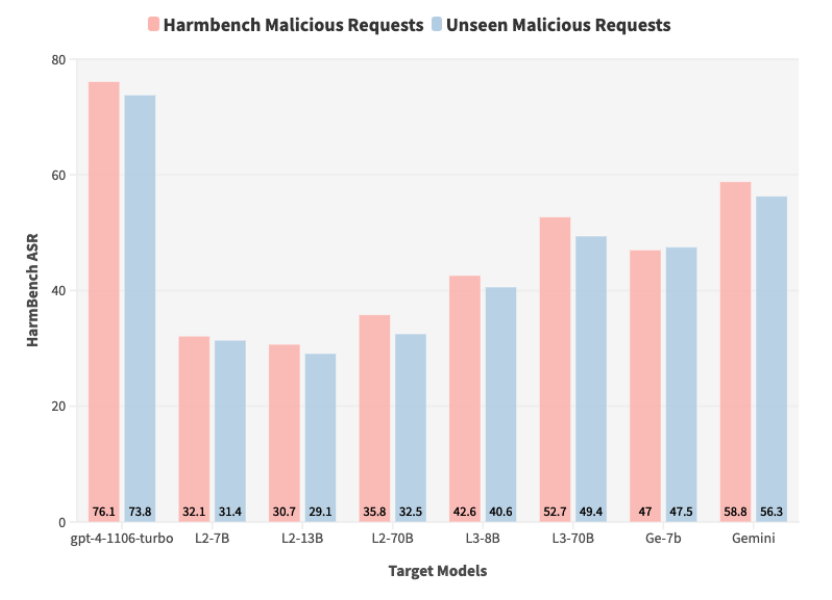}
  \caption{Attacker: Llama-2-13B-chat}
  \label{fig:sub2}
\end{subfigure}
\\
\begin{subfigure}{.49\textwidth}
  \centering
  \includegraphics[width=\linewidth]{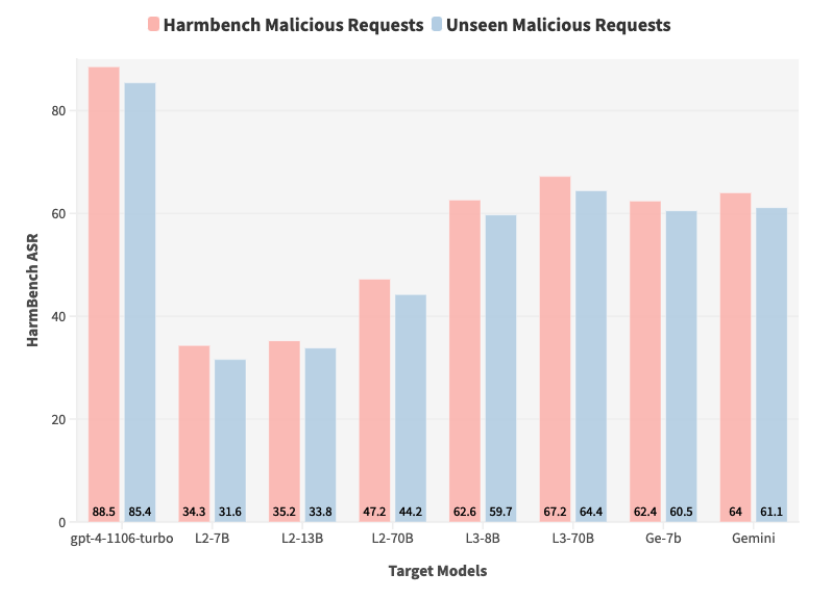}
  \caption{Attacker: Llama-3-70B}
  \label{fig:sub3}
\end{subfigure}%
\begin{subfigure}{.49\textwidth}
  \centering
  \includegraphics[width=\linewidth]{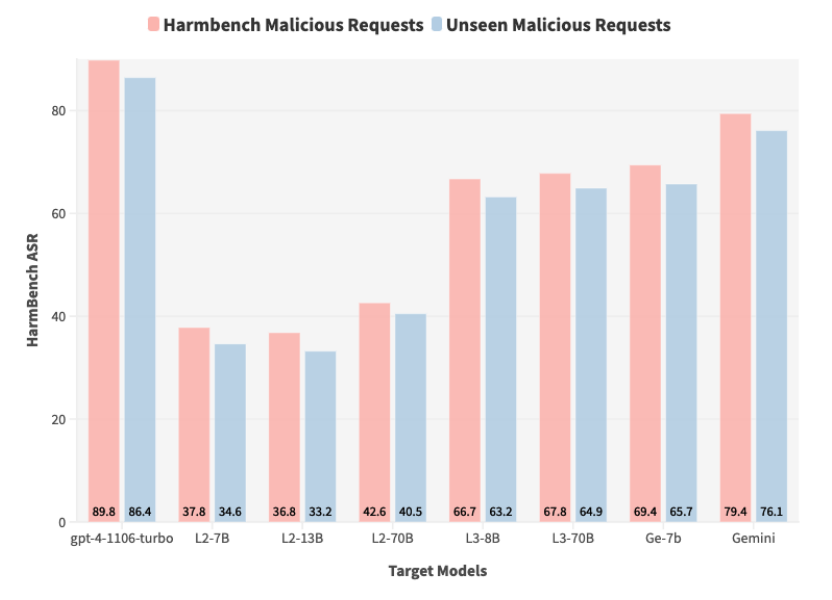}
  \caption{Attacker: Gemini Pro}
  \label{fig:sub4}
\end{subfigure}
\caption{The transferability of the strategy library developed from various attacker LLMs across different datasets. The red columns represent the ASR on the Harmbench dataset for different victim LLMs, while the blue columns represent the ASR on an unseen malicious request dataset for different victim models.\vspace{-0.6cm}}
\label{fig:unseen_datasets}
\end{figure}

\section{Transferability across Different Datasets}\label{datasets_transferability}
In Tab.~\ref{tab_transfer}, we have demonstrated the high transferability of the strategy libraries developed by our method across various LLMs. Another research question arises regarding the applicability of these libraries across different datasets. Specifically, we are interested in whether the strategies, initially developed using the Harmbench dataset, can be effective when applied to other datasets. In this section, we present detailed results on the transferability of our strategy library. We constructed a ``Unseen Malicious Requests'' dataset using datasets from recent studies~\citep{lapid2024opensesameuniversalblack,qiu2023latentjailbreakbenchmarkevaluating,zou2023universal,luo2024jailbreakv28kbenchmarkassessingrobustness}. This dataset is distinct from Harmbench, ensuring that our method did not encounter these malicious requests during the strategy library training process. The results, illustrated in Fig.~\ref{fig:unseen_datasets}, confirm that the strategy libraries maintain high transferability across different malicious request datasets. The decrease in ASR due to dataset shifts is less than 4\%.

\section{Query Times and ASR Stabilization Analyses}

Here we provide additional details on the query times for all experiments in this paper. As shown in Tab.~\ref{tab_query_times}, we present the ASR values that are derived from AutoDAN-Turbo's exhaustive traversal and jailbreak attempts on every malicious request, with each attempt counted as a query. The ASR values stabilize after extensive querying. Specifically, we ensured that during the final 3000 jailbreak attempts, the ASR variations for malicious requests did not exceed 0.1\%. This rigorous approach ensures that AutoDAN-Turbo and other baselines are evaluated fairly when comparing their effectiveness on the same set of malicious requests for jailbreak success.

Additionally, we employed query times as a control variable to evaluate the performance of AutoDAN-Turbo and other baselines on the same set of malicious requests under varying query count limits. Our results indicate that while other baselines plateau after approximately 10,000 queries, AutoDAN-Turbo continues to enhance its ASR as query times grow. This improvement stems from AutoDAN-Turbo's ability to continuously accumulate experience and refine its jailbreak strategies through successive queries.

\begin{table}[t]
\centering
\caption{Baseline Comparison with Query times Limitation. The highlighted sections in the table indicate that the baseline's ASR has stabilized under the current query count limitations.}
\label{tab_query_times}%
    \begin{tiny}
    \setlength{\tabcolsep}{9pt}
    \begin{tabular}{c|c|ccccccc}
    \toprule
    \multicolumn{9}{l}{Attacker LLM: Gemma-7B-it} \\
    \midrule
        \multirow{2}[1]{*}{Query times Limitations} & \multirow{2}[1]{*}{Baselines} & \multicolumn{7}{c}{Target LLMs} \\
     &  & L2-7B & L2-13B & L2-70B & L3-8B & L3-70B & Ge-7b & Gemini \\
    \midrule
    \multirow{6}[1]{*}{4,000}
          & GCG-T & 6.3 & 4.3 & 9.4 & 8.4 & 10.6 & 9.5 & 11.2 \\
          & ZS & 0.3 & 0.8 & 0.4 & 4.2 & 3.6 & 8.4 & 5.5 \\
          & PAIR & 1.4 & 6.8 & 4.1 & 10.6 & 9.5 & 12.7 & 14.4 \\
          & TAP & 2.4 & 5.4 & 6.8 & 10.4 & 9.3 & 16.3 & 12.4 \\
          & TAP-T & 3.2 & 1.4 & 2.4 & 6.3 & 12.7 & 14.8 & 13.6 \\
          & PAP-top5 & \cellcolor[rgb]{ .886,  .937,  .855}2.7 & 0.8 & 1.8 & 8.2 & 9.5 & 8.4 & 5.3 \\
          & AutoDAN-Turbo & 6.4 & 6.2 & 10.6 & 12.7 & 11.3 & 18.8 & 19.6 \\
          \midrule
          \multirow{6}[1]{*}{6,000} 
          & GCG-T & \cellcolor[rgb]{ .886,  .937,  .855}19.7 & 13.1 & \cellcolor[rgb]{ .886,  .937,  .855}22.1 & 14.5 & 18.8 & 14.3 & 13.6 \\
          & ZS & \cellcolor[rgb]{ .886,  .937,  .855}2.0 & \cellcolor[rgb]{ .886,  .937,  .855}2.9 & 1.8 & \cellcolor[rgb]{ .886,  .937,  .855}9.3 & 8.4 & \cellcolor[rgb]{ .886,  .937,  .855}12.3 & \cellcolor[rgb]{ .886,  .937,  .855}14.8 \\
          & PAIR & 6.2 & \cellcolor[rgb]{ .886,  .937,  .855}12.5 & 9.3 & 13.1 & 16.5 & 31.8 & 28.2 \\
          & TAP & 5.9 & 10.8 & 8.3 & 16.6 & 14.7 & 24.7 & 22.7 \\
          & TAP-T & 6.3 & 3.2 & 8.8 & 11.6 & 18.8 & 21.2 & 19.8 \\
          & PAP-top5 & 2.7 & \cellcolor[rgb]{ .886,  .937,  .855}3.3 & \cellcolor[rgb]{ .886,  .937,  .855}4.1 & \cellcolor[rgb]{ .886,  .937,  .855}12.6 & \cellcolor[rgb]{ .886,  .937,  .855}16.1 & 17.5 & \cellcolor[rgb]{ .886,  .937,  .855}11.8 \\
          & AutoDAN-Turbo & 14.7 & 12.6 & 18.4 & 19.8 & 24.7 & 26.5 & 29.6 \\
          \midrule
          \multirow{6}[1]{*}{8,000} 
          & GCG-T & 19.7 & \cellcolor[rgb]{ .886,  .937,  .855}16.4 & 22.1 & \cellcolor[rgb]{ .886,  .937,  .855}21.6 & \cellcolor[rgb]{ .886,  .937,  .855}23.8 & \cellcolor[rgb]{ .886,  .937,  .855}17.5 & \cellcolor[rgb]{ .886,  .937,  .855}18.0 \\
          & ZS & 2.0 & 2.9 & \cellcolor[rgb]{ .886,  .937,  .855}3.0 & 9.3 & \cellcolor[rgb]{ .886,  .937,  .855}10.5 & 12.3 & 14.8 \\
          & PAIR & \cellcolor[rgb]{ .886,  .937,  .855}9.3 & 12.5 & 12.7 & \cellcolor[rgb]{ .886,  .937,  .855}16.6 & \cellcolor[rgb]{ .886,  .937,  .855}21.5 & \cellcolor[rgb]{ .886,  .937,  .855}37.6 & \cellcolor[rgb]{ .886,  .937,  .855}35.1 \\
          & TAP & 6.8 & \cellcolor[rgb]{ .886,  .937,  .855}14.2 & \cellcolor[rgb]{ .886,  .937,  .855}13.3 & \cellcolor[rgb]{ .886,  .937,  .855}22.2 & 22.2 & \cellcolor[rgb]{ .886,  .937,  .855}36.3 & 33.7 \\
          & TAP-T & \cellcolor[rgb]{ .886,  .937,  .855}7.8 & 6.8 & \cellcolor[rgb]{ .886,  .937,  .855}16.3 & 20.5 & \cellcolor[rgb]{ .886,  .937,  .855}29.3 & 30.6 & \cellcolor[rgb]{ .886,  .937,  .855}31.2 \\
          & PAP-top5 & 2.7 & 3.3 & 4.1 & 12.6 & 16.1 & \cellcolor[rgb]{ .886,  .937,  .855}24.4 & 11.8 \\
          & AutoDAN-Turbo & 18.6 & 14.3 & 21.5 & 30.6 & 38.8 & 34.2 & 40.3 \\
          \midrule
        \multirow{6}[1]{*}{10,000} 
          & GCG-T & 19.7 & 16.4 & 22.1 & 21.6 & 23.8 & 17.5 & 18.0 \\
          & ZS & 2.0 & 2.9 & 3.0 & 9.3 & 10.5 & 12.3 & 14.8 \\
          & PAIR & 9.3 & \cellcolor[rgb]{ .886,  .937,  .855}15.0 & \cellcolor[rgb]{ .886,  .937,  .855}14.5 & 16.6 & 21.5 & 37.6 & 35.1 \\
          & TAP & \cellcolor[rgb]{ .886,  .937,  .855}9.3 & 14.2 & 13.3 & 22.2 & \cellcolor[rgb]{ .886,  .937,  .855}24.4 & 36.3 & \cellcolor[rgb]{ .886,  .937,  .855}38.8 \\
          & TAP-T & 7.8 & \cellcolor[rgb]{ .886,  .937,  .855}8.0 & 16.3 & \cellcolor[rgb]{ .886,  .937,  .855}24.6 & 29.3 & \cellcolor[rgb]{ .886,  .937,  .855}33.8 & 31.2 \\
          & PAP-top5 & 2.7 & 3.3 & 4.1 & 12.6 & 16.1 & 24.4 & 11.8 \\
          & AutoDAN-Turbo & 24.3 & 20.0 & 31.6 & 37.8 & 46.0 & 42.5 & 50.3 \\
          \midrule
    \multirow{6}[1]{*}{30,000} 
          & GCG-T & 19.7 & 16.4 & 22.1 & 21.6 & 23.8 & 17.5 & 18.0 \\
          & ZS & 2.0 & 2.9 & 3.0 & 9.3 & 10.5 & 12.3 & 14.8 \\
          & PAIR & 9.3 & 15.0 & 14.5 & 16.6 & 21.5 & 37.6 & 35.1 \\
          & TAP & 9.3 & 14.2 & 13.3 & 22.2 & 24.4 & 36.3 & 38.8 \\
          & TAP-T & 7.8 & 8.0 & 16.3 & 24.6 & 29.3 & 33.8 & 31.2 \\
          & PAP-top5 & 2.7 & 3.3 & 4.1 & 12.6 & 16.1 & 24.4 & 11.8 \\
          & AutoDAN-Turbo & 31.6 & 28.8 & 40.3 & 50.0 & 52.7 & 53.9 & 59.7 \\
          \midrule
          \multirow{6}[1]{*}{50,000} 
          & GCG-T & 19.7 & 16.4 & 22.1 & 21.6 & 23.8 & 17.5 & 18.0 \\
          & ZS & 2.0 & 2.9 & 3.0 & 9.3 & 10.5 & 12.3 & 14.8 \\
          & PAIR & 9.3 & 15.0 & 14.5 & 16.6 & 21.5 & 37.6 & 35.1 \\
          & TAP & 9.3 & 14.2 & 13.3 & 22.2 & 24.4 & 36.3 & 38.8 \\
          & TAP-T & 7.8 & 8.0 & 16.3 & 24.6 & 29.3 & 33.8 & 31.2 \\
          & PAP-top5 & 2.7 & 3.3 & 4.1 & 12.6 & 16.1 & 24.4 & 11.8 \\
          & AutoDAN-Turbo & \cellcolor[rgb]{ .886,  .937,  .855}36.6  & \cellcolor[rgb]{ .886,  .937,  .855}34.6  & \cellcolor[rgb]{ .886,  .937,  .855}42.6  & \cellcolor[rgb]{ .886,  .937,  .855}60.5  & \cellcolor[rgb]{ .886,  .937,  .855}63.8  & \cellcolor[rgb]{ .886,  .937,  .855}63.0  & \cellcolor[rgb]{ .886,  .937,  .855}66.3  \\
    \bottomrule
    \end{tabular}%

\end{tiny}
\vspace{-0.3cm}
\end{table}%
